# Supplementary material for: "Average" Approximates "First Principal Component"? An Empirical Analysis on Representations from Neural Language Models
Source: arXiv:2104.08673 source file (2022-02-07)
Supplement: Supplementary file 1 [file appendix.tex]

% %
% % File acl2020.tex
% %
% %% Based on the style files for ACL 2020, which were
% %% Based on the style files for ACL 2018, NAACL 2018/19, which were
% %% Based on the style files for ACL-2015, with some improvements
% %%  taken from the NAACL-2016 style
% %% Based on the style files for ACL-2014, which were, in turn,
% %% based on ACL-2013, ACL-2012, ACL-2011, ACL-2010, ACL-IJCNLP-2009,
% %% EACL-2009, IJCNLP-2008...
% %% Based on the style files for EACL 2006 by 
% %%e.agirre@ehu.es or Sergi.Balari@uab.es
% %% and that of ACL 08 by Joakim Nivre and Noah Smith

% \documentclass[11pt,a4paper]{article}
% \usepackage[]{emnlp2021}
% \usepackage{times}
% \usepackage{latexsym}
% \renewcommand{\UrlFont}{\ttfamily\small}

% % This is not strictly necessary, and may be commented out,
% % but it will improve the layout of the manuscript,
% % and will typically save some space.
% \usepackage{microtype}

% \usepackage{tabularx, booktabs}
% \usepackage{multirow}
% \usepackage[inline]{enumitem}
% \usepackage{wrapfig}
% \usepackage{array}
% \usepackage{diagbox}
% \usepackage{xspace}
% \usepackage{url}
% \usepackage{graphicx}
% \usepackage{subfigure}
% \usepackage[noend,ruled]{algorithm2e}
% \usepackage{amsmath}
% \usepackage{amssymb,mathtools,bm,etoolbox}
% % \usepackage{floatrow}

% % \aclfinalcopy % Uncomment this line for the final submission
% %\def\aclpaperid{***} %  Enter the acl Paper ID here

% %\setlength\titlebox{5cm}
% % You can expand the titlebox if you need extra space
% % to show all the authors. Please do not make the titlebox
% % smaller than 5cm (the original size); we will check this
% % in the camera-ready version and ask you to change it back.

% \newcommand\BibTeX{B\textsc{ib}\TeX}


% \newcommand{\TODO}[1]{\textcolor{red}{[TODO: {#1}]}}
% \newcommand{\ZW}[1]{\textcolor{blue}{[ZW: {#1}]}}
% \newcommand{\jingbo}[1]{\textcolor{blue}{[\textbf{Jingbo}: {#1}]}}
% \newcommand{\smallsection}[1]{\noindent{\textbf{#1.}}}
% % \newfloatcommand{capbtabbox}{table}[][\FBwidth]



% \begin{document}

% \appendix
% \input{8-appendix}

% \end{document}
